# Supplementary material for: Iterative subspace algorithms for finite-temperature solution of Dyson equation
Source: arXiv:2112.08890 source file (2021-12-16)
Supplement: Supplementary file 1 [file SI.pdf]

# Iterative subspace algorithms for finite-temperature solution of Dyson equation

Pavel Pokhilko,[1] Chia-Nan Yeh,[2] and Dominika Zgid[1,2]

[1]*Department of Chemistry, University of Michigan, Ann Arbor, Michigan 48109, USA*

[2]*Department of Physics, University of Michigan, Ann Arbor, Michigan 48109, USA*

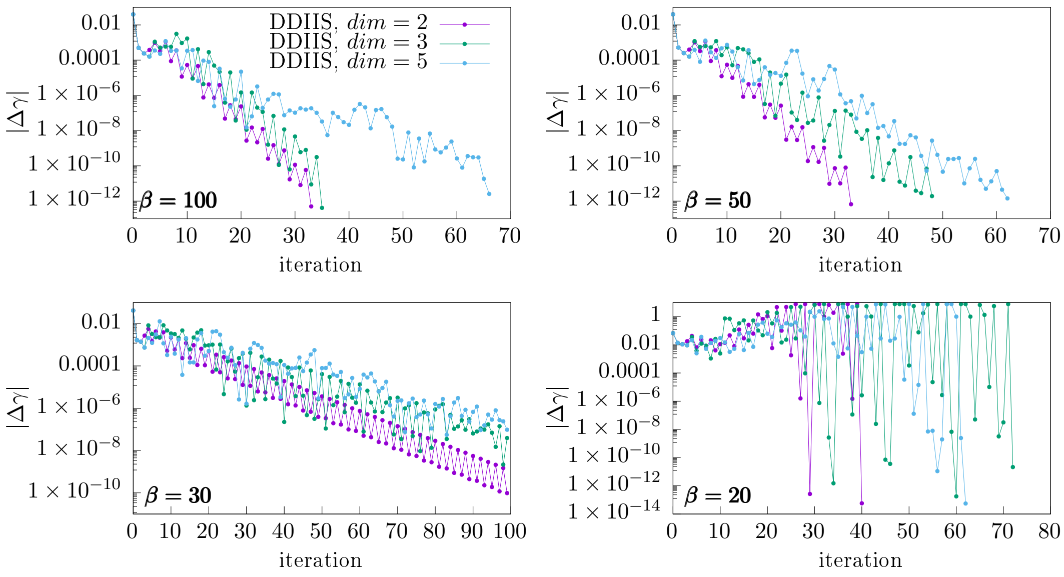


FIG. S1: Convergence of DIIS for GW calculations for a Be atom for a range of inverse temperatures $\beta$. Different values of the subspace size are shown as *dim*. The step size was not restricted.

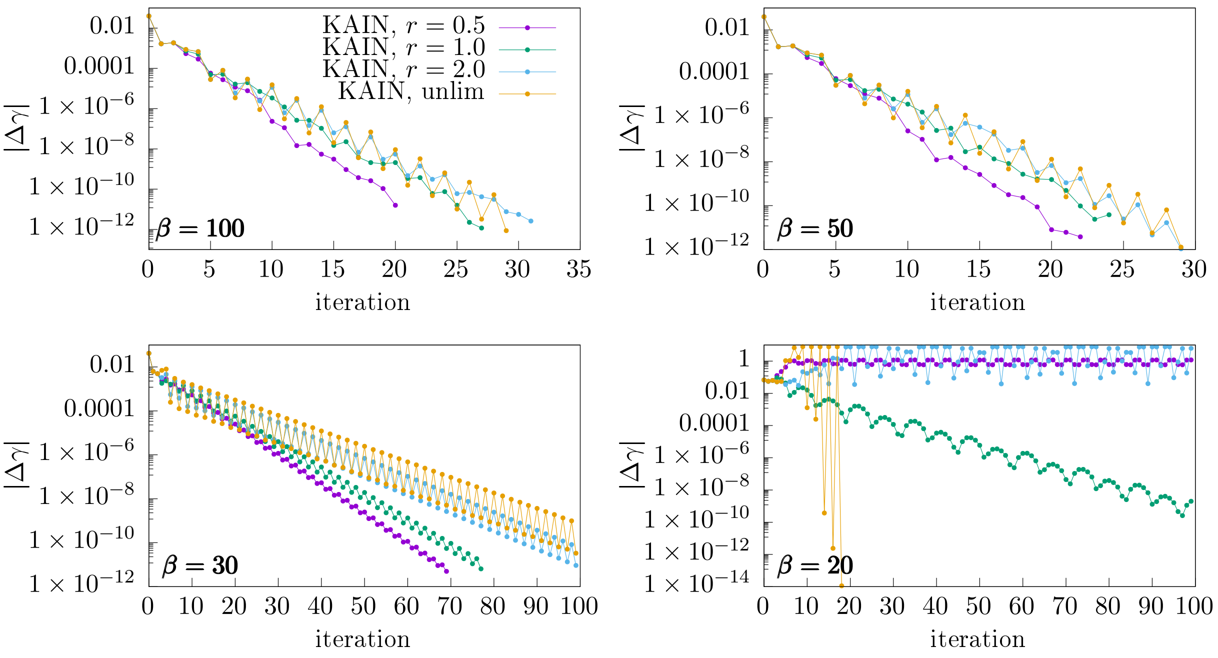


FIG. S2: The convergence of KAIN for GW calculations for a Be atom for a range of inverse temperatures $\beta$. Different values of the step restriction parameter $r$ are shown. The calculations where the step restriction has not been applied, are labeled as *unlim*. The subspace size is 2.

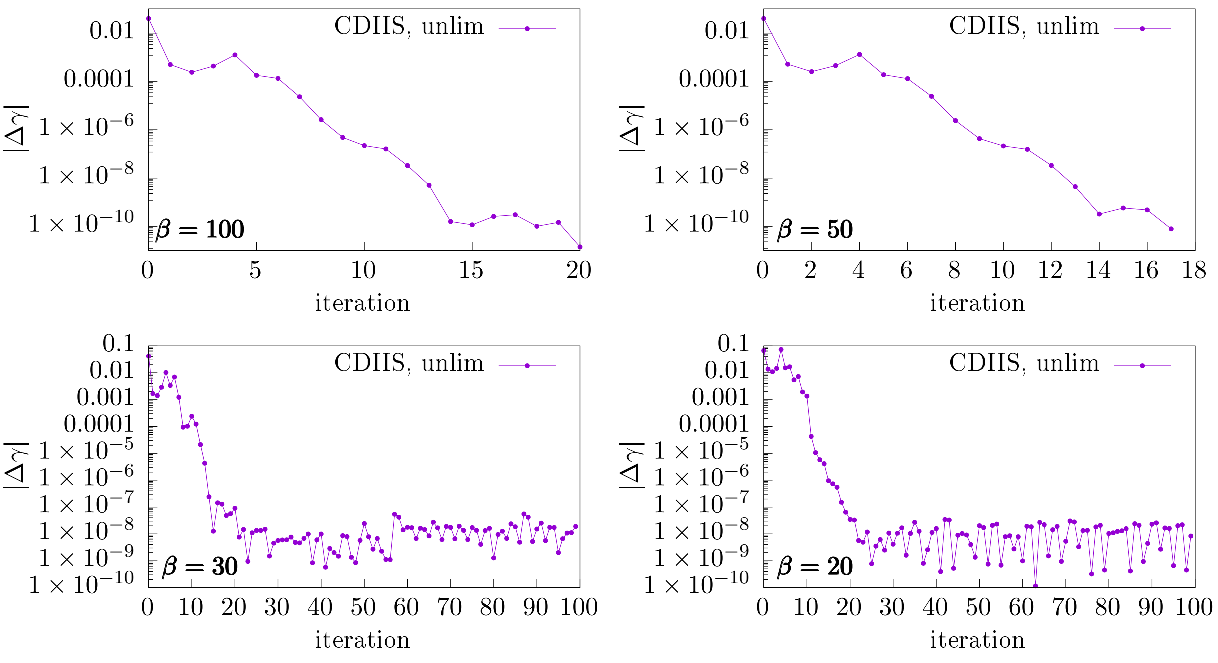


FIG. S3: The convergence of CDIIS for GW calculations for a Be atom for a range of inverse temperatures $\beta$. The size of the subspace is 2. The step size was not restricted.

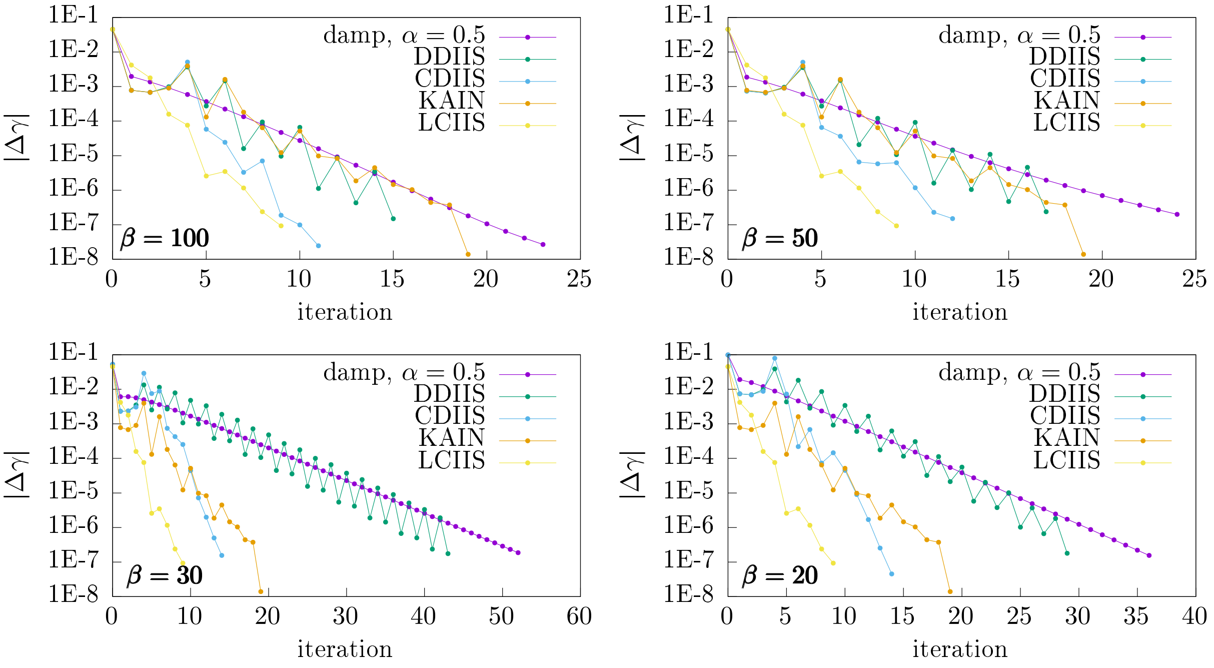


FIG. S4: The convergence of iterative algorithms for GW calculations for a Mg atom for a range of inverse temperatures $\beta$. The size of the subspace is 2 for all subspace algorithms. The step size was not restricted. The chemical potential is optimized at each iteration to produce a correct number of electrons present in the ground state.

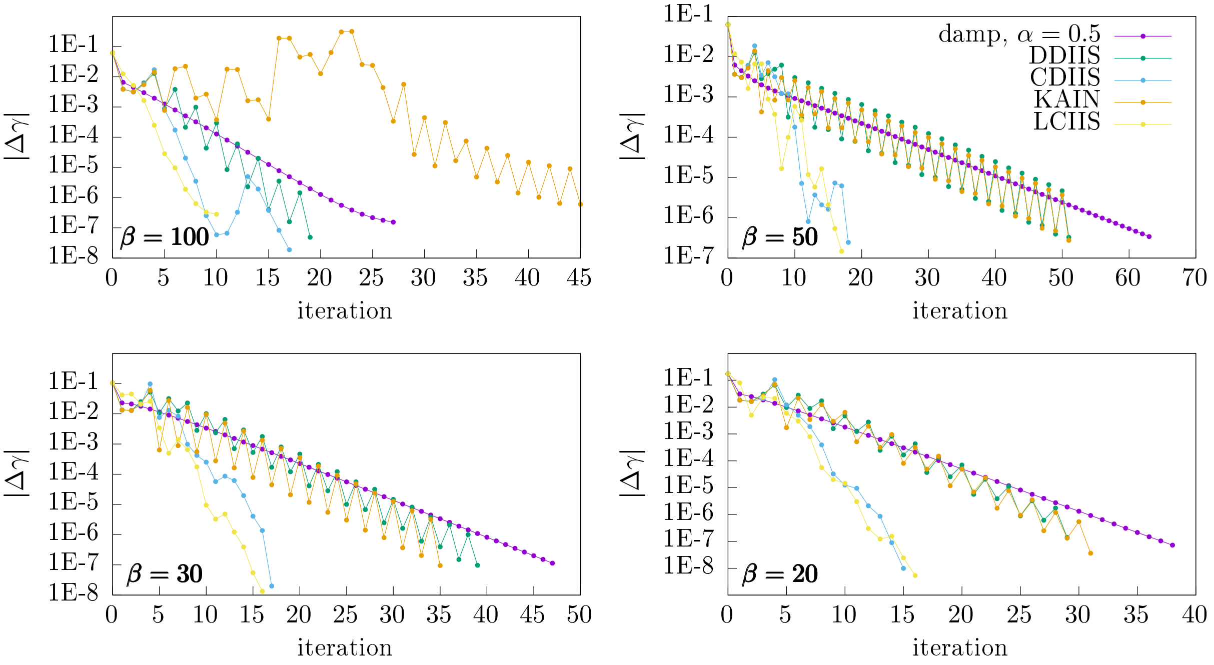


FIG. S5: The convergence of iterative algorithms for GW calculations for a Ca atom for a range of inverse temperatures $\beta$. The size of the subspace is 2 for all subspace algorithms. The step size was not restricted. The chemical potential is optimized at each iteration to produce a correct number of electrons present in the ground state.

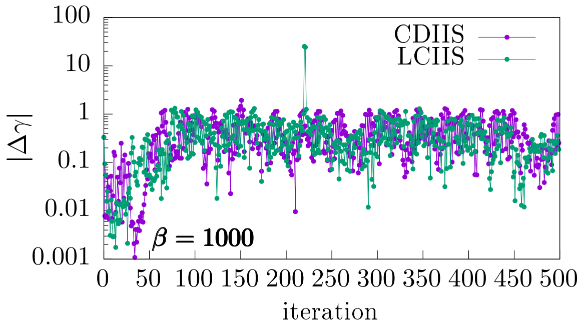


FIG. S6: The convergence of CDIIS and LCIIS for GF2 calculations for a stretched $H_2$ molecule from a zero-temperature RHF guess. The size of the subspace is 2 for all subspace algorithms. The step size was not restricted. The chemical potential is optimized at each iteration to produce a correct number of electrons present in the ground state.

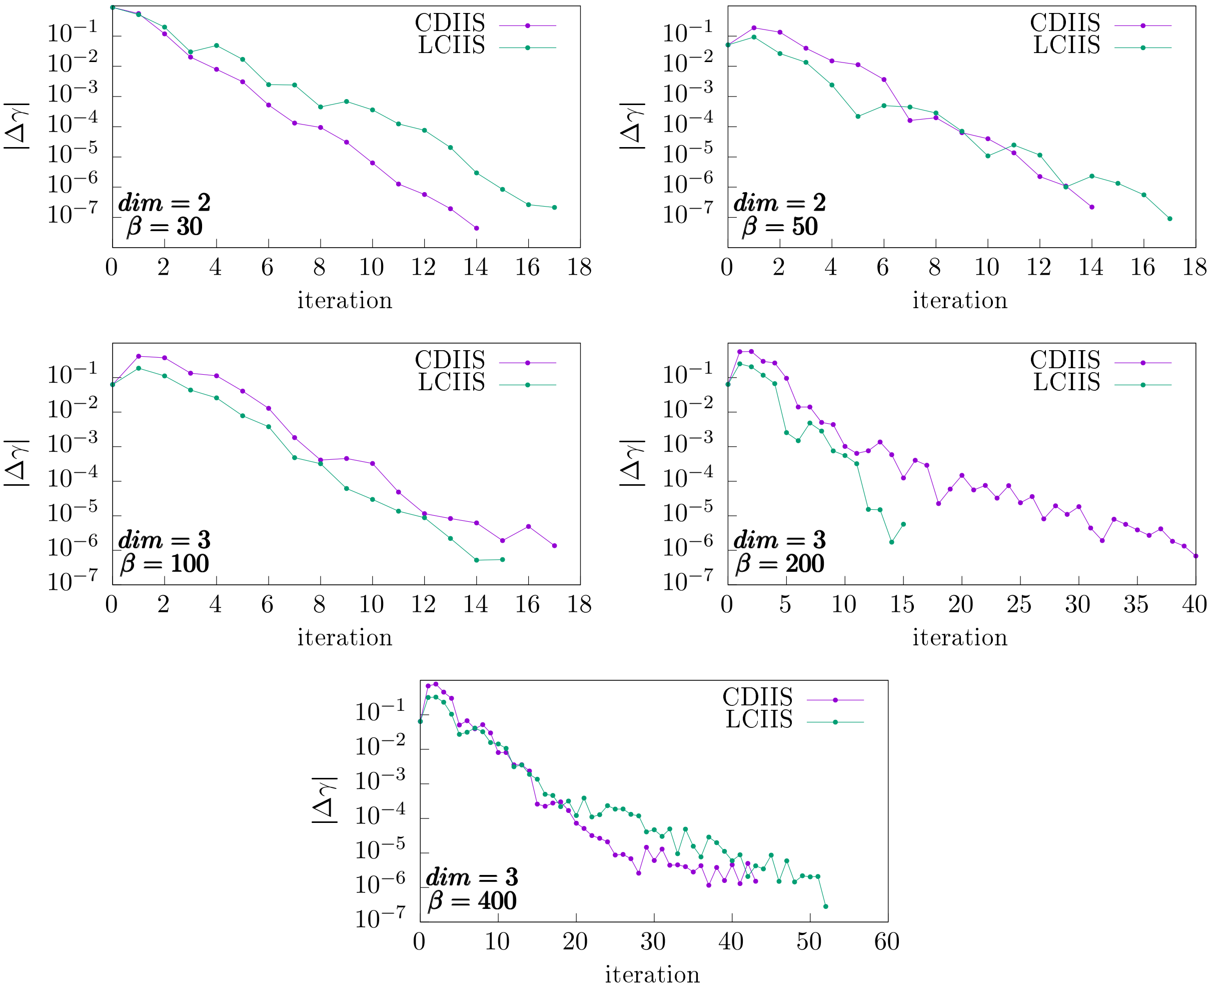


FIG. S7: The Convergence of CDIIS and LCIIS for RGF2 calculations for a stretched $H_8$ cube for different temperatures. The initial guesses for each runs are taken either from the finite-temperature HF ($\beta = 30$) or from the RGF2 at higher temperature (all other graphs). The subspace size is indicates in each of the graphs as *dim*.

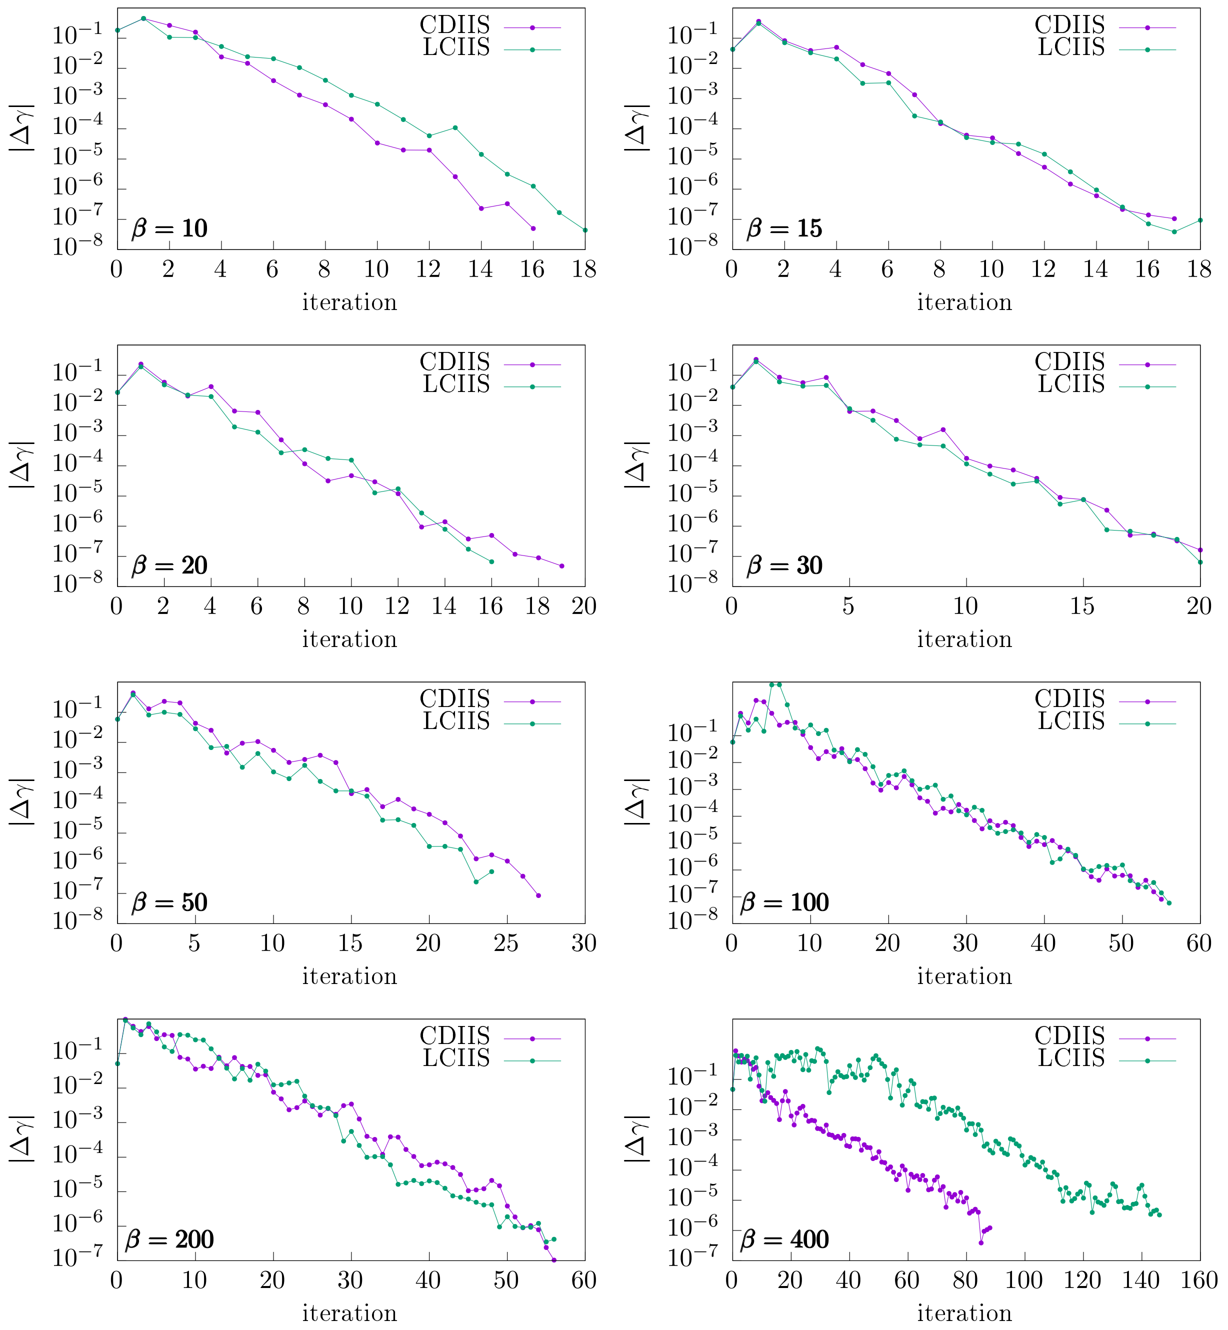


FIG. S8: The convergence of CDIIS and LCIIS for RGF2 calculations on a stretched $N_2$ for different temperatures. The initial guesses for each runs are taken either from the finite-temperature HF ($\beta = 10$) or from the RGF2 at higher temperature (all other graphs). The subspace size is 5.
